# Supplementary material for: Intelligent Collision Management in Dynamic Environments for Human-Centered Robots
Source: arXiv:1711.02290 source file (2017-11-07)
Supplement: Supplementary file 1 [file chapter-appendix4.tex]

\chapter{Whole-body operational space control for underactuated and unconstrained systems}
\label{sec:TH}
The dynamic system including some unactuated joints and constraints can be express as the following constrained dynamic equation.
\begin{align}
A \ddot{q} + N_c^T \, bg = \left(U N_c \right)^T \tau
\end{align}
On the given system, we can define a task space which has a task coordinate, $x$ which has the following derivative relationship with the generalized coordinate,
\begin{align}
\dot{x} = J \dot{q},
\end{align}
and the task space dynamic equation can be expressed as follows.
\begin{align}
\ddot{x} - \dot{J}\dot{q} + J A^{-1} N_c^T \, bg = J A^{-1} \left( U N_c \right)^T \tau\label{eq:const_dyn}
\end{align}
Before dealing with unactuated joints, we can assume all the joints in the system can be actuated with a force/torque vector, $\tau^\prime$ as follows.
\begin{align}
\ddot{x} - \dot{J}\dot{q} + J A^{-1} N_c^T \, bg = J A^{-1} N_c^T \tau^\prime
\end{align}
If the task Jacobian, $J$ has a full row rank, then the system can accelerate to any directions in the constrained manifold. Also, if the task Jacobian is not a symmetric matrix, more than one solution for a given task acceleration, and we can choose one solution which is dynamically consistent. 

Given $\tau^{\prime}$ we may find an input that generates the same task acceleration to that of $\tau_{\prime}$ if the underactuated system is fully controllable in the constrained manifold. Unless the desired task acceleration cannot be achieved and dynamically consistent minimum error input can be derived as follows.
\begin{align}
\tau = \overline{U N_c} \tau^\prime\label{eq:tau_p}
\end{align}

By substituting Eq. (\ref{eq:tau_p}) to the constrained dynamics in Eq. (\ref{eq:const_dyn}),
\begin{align}
\ddot{x} - \dot{J}\dot{q} + J A^{-1} N_c^T \, bg = J A^{-1} \left( U N_c \right)^T \overline{U N_c}^T \tau^\prime \label{eq:const_dyn2}
\end{align}
Defining $N_c^\prime \triangleq \overline{U N_c} U N_c$, we can derive a new constrained dynamics as follows.
\begin{align}
\ddot{x} - \dot{J}\dot{q} + J A^{-1} N_c^T \, bg = J A^{-1} N_c^{\prime\, T} \tau^\prime \label{eq:const_dyn2}
\end{align}
If the rank of $U N_c$ is equal to that of $N_c$ which means the unactuated joints are fully constrained. 

The dynamically consistent control input for a desired task acceleration, $\ddot{x}_{des}$ can be derived as follows.
\begin{align}
\tau^\prime = J^T \left( J A^{-1} N_c^{\prime\, T} J^T \right)^+ \left( \ddot{x}_{des} - \dot{J} \dot{q} + J A^{-1} N_c^T bg  \right)
\end{align}

$N_c^{\prime}$ has the same property to that of $N_c$ as follows.
\begin{align}
N_c^{\prime\, 2} &= N_c^\prime \\
A^{-1} N_c^{\prime\, T} &= N_c^\prime A^{-1}
\end{align}
